# Supplementary material for: The 26 Wilf-equivalence classes of length five quasi-consecutive patterns
Source: arXiv:1609.04626 source file (2018-10-22)
Supplement: Supplementary file 1 [file appendix.tex]

\appendix
\section{\\Title of Appendix A} \label{App:AppendixA}

    Here we explain in detail why our results fully complete the Wilf-equivalence classification for vincular patterns of the form $\sigma_1\sigma_2\sigma_3\sigma_4-\sigma_5$
\begin{table}
\centering
\begin{tabular}{ |c||c| } 
    \hline
    1 & 1254-3, 1354-2 \\ \hline
    2 & 1453-2, 1543-2 \\ \hline
    3 & 2135-4, 2145-3 \\ \hline
    4 & 1534-2 \\ \hline
    5 & 2315-4 \\ \hline
    6 & 1243-5, 1253-4, 2134-5, 2354-1, 3145-2, 3245-1 \\ \hline
    7 & 3125-4, 3215-4 \\ \hline
    8 & 1435-2 \\ \hline
    9 & 1523-4 \\ \hline
    10 & 3251-4 \\ \hline
    11 & 2154-3 \\ \hline
    12 & 1342-5, 1352-4, 1432-5, 1452-3, 1532-4, 1542-3, 2341-5, 2351-4, \\ 
     & 2431-5, 2451-3, 2453-1, 2531-4, 2541-3, 2543-1, 3124-5, 3214-5 \\ \hline
    13 & 2153-4, 3154-2 \\ \hline
    14 & 2513-4 \\ \hline
    15 & 1524-3 \\ \hline
    16 & 2415-3 \\ \hline
    17 & 1325-4 \\ \hline
    18 & 1423-5, 2314-5, 2534-1, 3241-5 \\ \hline
    19 & 2143-5, 3254-1 \\ \hline
    20 & 3152-4 \\ \hline
    21 & 1425-3 \\ \hline
    22 & 1324-5, 2435-1 \\ \hline
    23 & 2514-3 \\ \hline
    24 & 2413-5, 3142-5 \\ \hline
    25 & 1235-4, 1245-3, 1345-2 \\ \hline
    26 & 1234-5, 2345-1 \\ \hline
\end{tabular}
\caption{The complete list of Wilf-equivalence classes for patterns of the form $\sigma_1\sigma_2\sigma_3\sigma_4-\sigma_5.$  Complements are not included.  Our results show that everything in columns 1, 2, 3, 7, 12, and 13 are Wilf-equivalent.}
\end{table}
